# Supplementary material for: User or Labor: An Interaction Framework for Human-Machine Relationships in NLP
Source: arXiv:2211.01553 source file (2022-11-03)
Supplement: Supplementary file 2 [file Sec9.Appendix.tex]

%\section{Appendix}
%\label{sec:appendix}

% \subsection{Correlation between interaction properties and relationships}
% \input{Tables/table1.tex}


% \begin{figure*}[!h]
% \centering
% \includegraphics[width=1\textwidth]{Figures/Properties_Relationships.pdf}
% \caption{Human-machine Relationships Mapping Interaction Properties
% \label{fig:relationship_mapping}}
% \end{figure*}

% Figure \ref{fig:relationship_mapping} shows some trends of interactions: Human-Leading relationship usually happens with sequential interactions;  Machine-Leading relationship uses more GUI and has iterative interaction; Human-Machine Collaborators mainly use NUI; Human-Teacher, Machine-Learner relationship usually happens iteratively as well.
